# Supplementary material for: Automated Creation of Digital Cousins for Robust Policy Learning
Source: arXiv:2410.07408 source file (2024-10-19)
Supplement: Supplementary file 2 [file rebuttal_acdc_failure_cases.tex]

\begin{figure}[t]
    \centering
    \includegraphics[width=\textwidth]
    {example-image-a}
    \caption{Visualized failure cases for \acdc.}
    \label{fig:supp-rebuttal_acdc_failure_cases}
    \vspace{-0.1in}
\end{figure}
